# Supplementary material for: Femtojoule-scale all-optical latching and modulation via cavity nonlinear optics
Source: arXiv:1305.1077 ancillary file (2013-08-06)
Supplement: Supplementary file 1 [file supplementary_info.pdf]

# Femtojoule-scale all-optical latching and modulation via cavity nonlinear optics

Yeong-Dae Kwon, Michael A. Armen, and Hideo Mabuchi\*

*Edward L. Ginzton Laboratory, Stanford University, Stanford, CA 94305*

(Dated: April 20, 2013)

---

\* Electronic address: hmabuchi@stanford.edu

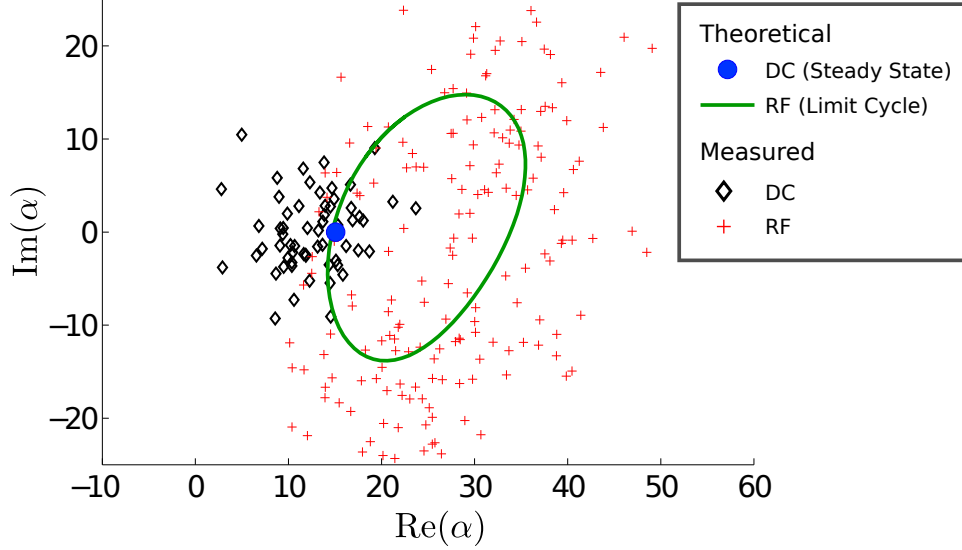

**Figure S1. Intracavity field states of the dc-rf latch depicted in Fig.3.** The measured dc and rf states of the latch are compared with theoretical predictions.  $\alpha$  is the complex amplitude of the coherent cavity field state. The measured data for the rf state plotted in the figure represent 25 cycles of oscillation, roughly 7 data points for each cycle. The width of the data spread matches the expected level of quantum noise on the heterodyne signal output, accounting for the quantum efficiency of the detector ( $\sim 20\%$ ) and the optical losses.

**Methods.** The most common way of measuring the complex amplitude of an optical field is heterodyne detection, where this field is interfered with a stable, frequency-detuned local oscillator, such that the information carried by the measured signal oscillates between that of the amplitude quadrature ( $\text{Re}\{\alpha\}$ ) and that of the phase quadrature ( $\text{Im}\{\alpha\}$ ) at the (fast) detuning frequency. Each value of the field quadrature is then extracted through rf demodulation of the heterodyne signal. In our case, however, such a scheme was not applicable because the intracavity field state we wanted to measure oscillates at a fast rate ( $\sim 23\text{MHz}$ ), comparable to the bandwidth of the detector ( $80\text{MHz}$ ).

For this reason, we use a slow heterodyne frequency ( $2\text{MHz}$ ) instead, so that we effectively measure only one quadrature value while the intracavity state undergoes several limit cycle oscillation. Assuming that the known limit cycle frequency remains constant, we define a set of points in time, spaced by the measured period of the limit cycle, such that the state of the system at each time is supposed to be on the same spot of the limit cycle. From this set of points, we select two points whose separation is close to the quarter period of the heterodyne measurement ( $125\text{ ns}$ ). Measurements made at these two points in time give us a pair of complementary quadrature values, which we then combine to create one complex amplitude data point, plotted in Fig.S1. We repeat this process over  $\sim 25$  limit cycle oscillations to create the complex phasor portrait displayed above.

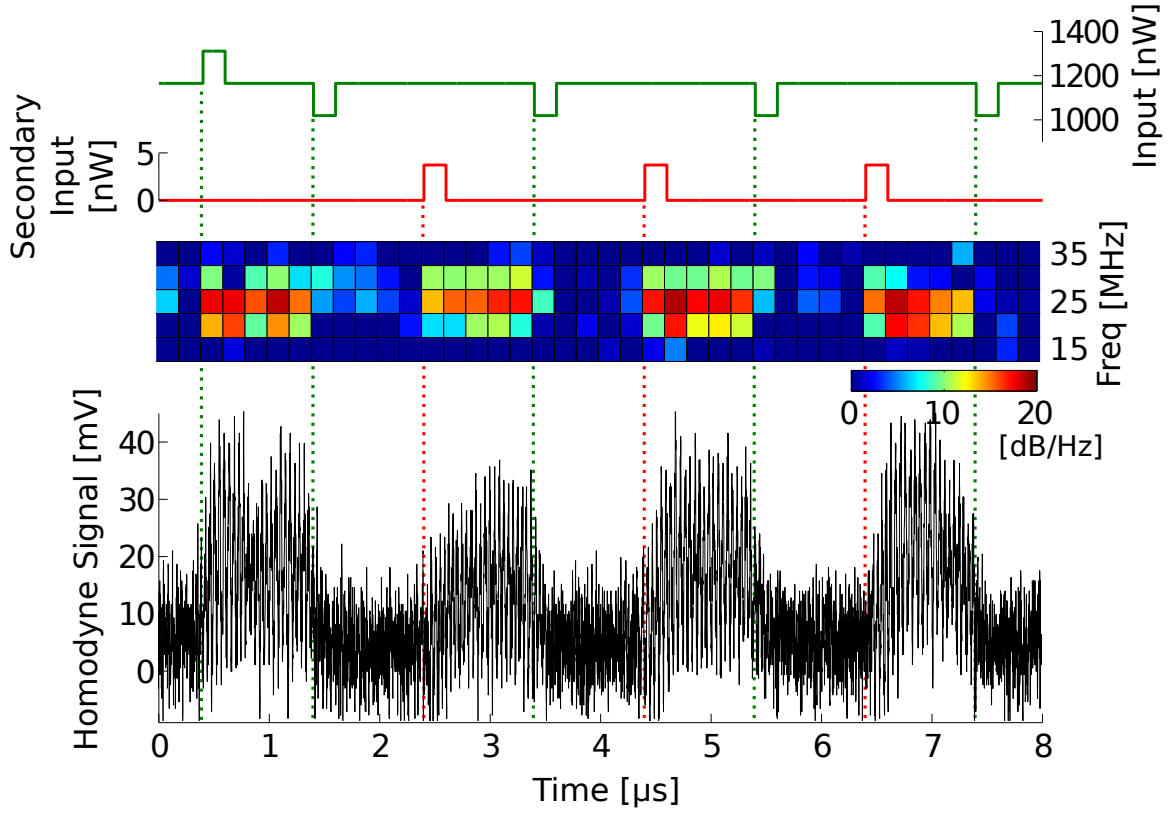

**Figure S2. Demonstration of the dc-rf latch switch-on operation using a sub-femtojoule secondary input pulse.** The parameters used are  $N_{\text{eff}} = 2100$ ,  $\Delta_C/2\pi = -20\text{MHz}$ ,  $\Delta_A/2\pi = 5\text{MHz}$ , same as in Fig.3. Here, we added a second input beam which has frequency  $\omega_{\text{las2}}$  where  $\omega_{\text{las2}} - \omega_{\text{las}} = -2\pi \cdot 23\text{MHz}$  and  $\omega_{\text{las2}} - \omega_{\text{cav}} = -2\pi \cdot 3\text{MHz}$ . The beating created by the two input beams matches the expected frequency of the limit cycle.

During the 0 - 2  $\mu\text{sec}$  segment shown above, the dc-rf latch was switched on and off by adding positive and negative pulses to the primary beam (shown in green), similar to what was demonstrated in Fig.3. In contrast, from 2 to 8  $\mu\text{sec}$  rf latching was initiated by applying pulses of the secondary beam (red) with energy  $4\text{nW} \times 0.2\mu\text{s} = 0.8\text{fJ}$  for each pulse. We have observed that at this energy level the pulses are able to switch the latch from the dc- to the rf-state reliably. Negative pulses of the primary beam were still used to reset the latch back to the dc-state and have it ready for subsequent switch-on pulses.
